# Supplementary material for: OPT-IML: Scaling Language Model Instruction Meta Learning through the Lens of Generalization
Source: arXiv:2212.12017 source file (2023-01-30)
Supplement: Supplementary file 1 [file appendix_header.tex]

\documentclass{article} % For LaTeX2e
% \usepackage{iclr2023_conference,times}
\usepackage{jmlr2e}

% Optional math commands from https://github.com/goodfeli/dlbook_notation.
\input{math_commands.tex}

\usepackage{hyperref}
\usepackage{url}
\usepackage{amssymb}
\usepackage{booktabs}
\usepackage{pifont}
\usepackage{xspace}
\usepackage{graphicx}
\usepackage{makecell}
\usepackage{xcolor,colortbl}
\usepackage{arydshln} % for dashed line in tables 
\usepackage{multirow}
\usepackage{longtable,tabu}
\usepackage{caption}
\usepackage{subcaption}
\usepackage{lscape}
\usepackage{longtable}


% models
\newcommand{\model}[2]{#1$_\textsc{#2}$}
\newcommand{\Oursf}{OPT-IML\includegraphics[scale=0.043]{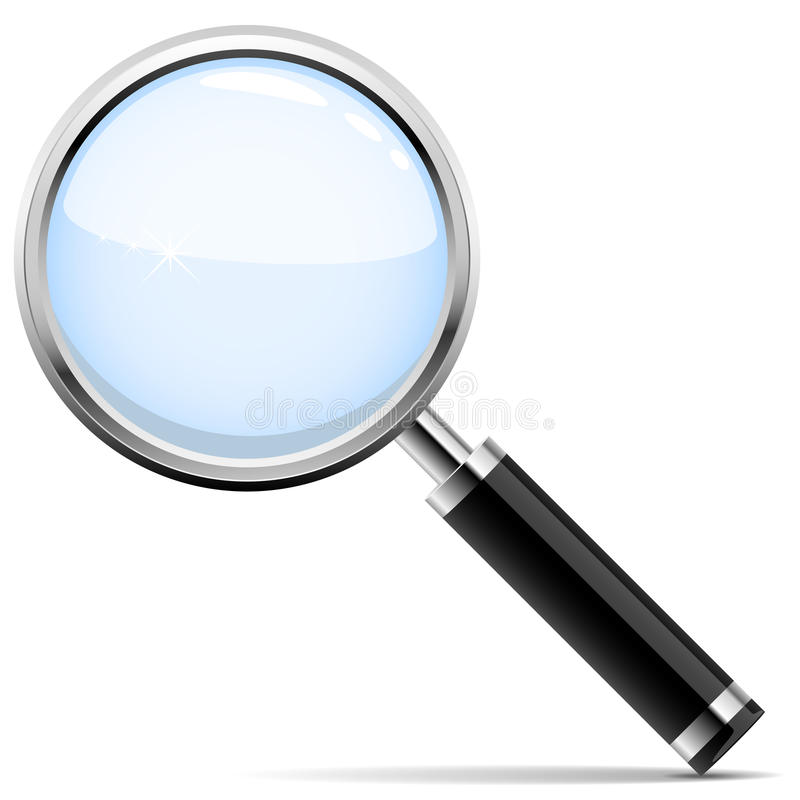}\xspace}
\newcommand{\OursLargeIcon}{OPT-IML\includegraphics[scale=0.068]{figures/lens.jpg}\xspace}
\newcommand{\Ours}{OPT-IML\xspace}
\newcommand{\OursB}{\Ours Bench\xspace}
\newcommand{\gptinstruct}{GPT3-Instruct\xspace}
\newcommand{\tfive}{\textsc{T5}\xspace}
\newcommand{\bart}{\textsc{BART}\xspace}
\newcommand{\tzero}{\textsc{T0}\xspace}
\newcommand{\tkinstruct}{T$k$-\textsc{Instruct}\space}

% benchmarks
\newcommand{\natins}{Super-NaturalInstructions\xspace}
\newcommand{\natinsShort}{SuperNatInst}
\newcommand{\promptsource}{PromptSource\xspace}
\newcommand{\crossfit}{CrossFit\xspace}
\newcommand{\flan}{FLAN\xspace}
\newcommand{\exmix}{ExMix\xspace}
\newcommand{\bb}{BB3 Dialogue\xspace}
\newcommand{\unifiedskg}{UnifiedSKG\xspace}
\newcommand{\bigbench}{BIG-bench\xspace}
\newcommand{\cotr}{Chain-of-thought Reasoning\xspace}
\newcommand{\cotrShort}{Reasoning\xspace}

% organizations
\newcommand{\bigscience}{BigScience}

\newcommand{\highest}[1]{\textbf{#1}}
\newcommand{\hide}[1]{}

\definecolor{tblue}{HTML}{174992}
\newcommand{\todo}[1]{\textcolor{red}{[\textbf{#1}]}}
\newcommand{\srini}[1]{{\color{blue} [Srini: {#1}]}}
\newcommand{\ram}[1]{{\color{purple} [Ram: {#1}]}}
\newcommand{\vic}[1]{\textcolor{teal}{[Victoria: {#1}]}}
\newcommand{\ves}[1]{\textcolor{green}{[Ves: {#1}]}}
\newcommand{\ping}[1]{\textcolor{orange}{[Ping: {#1}]}}
\newcommand{\daniel}[1]{\textcolor{orange}{[Daniel: {#1}]}}
\newcommand{\luke}[1]{\textcolor{violet}{[Luke: {#1}]}}

\newcommand{\zest}{\textsc{Zest}\xspace}

% writing hacks
\newcommand{\mask}{\texttt{[Mask]}}
\newcommand{\sep}{{\small\texttt{[Sep]}}}
\newcommand{\outlier}{$^{\dagger}$}
\newcommand{\outliertwo}{$^{\ddag}$}
\newcommand{\outlierthree}{$^{\star}$}
\newcommand{\textnewline}{\textbackslash n}

\definecolor{DarkGreen}{RGB}{30,130,30}
\newcommand{\cmark}{\textcolor{DarkGreen}{\ding{51}}}
\newcommand{\xmark}{\textcolor{red}{\ding{55}}}%

% example table hacks
\definecolor{antiquewhite}{rgb}{0.98, 0.92, 0.84}
\definecolor{airforceblue}{rgb}{0.36, 0.54, 0.66}
\definecolor{cadmiumgreen}{rgb}{0.0, 0.42, 0.24}
\definecolor{lightgray}{rgb}{0.83, 0.83, 0.83}
\definecolor{oldlace}{rgb}{0.99, 0.96, 0.9}
\extrafloats{1000}

\title{\OursLargeIcon: Extreme Multi-Task Scaling for Language Model Instruction Meta Tuning} % tentative. Suggestions by people: OPTuned, OPT=0, 0-PT, Meta-OPT

% Authors must not appear in the submitted version. They should be hidden
% as long as the \iclrfinalcopy macro remains commented out below.
% Non-anonymous submissions will be rejected without review.

% Author information can be set in various styles:
% For several authors from the same institution:
\author{Author 1 \and ... \and Author n \\
        \addr{Address line} \\ ... \\ \addr{Address line}}
% if the names do not fit well on one line use
%         Author 1 \\ {\bf Author 2} \\ ... \\ {\bf Author n} \\
% To start a seperate ``row'' of authors use \AND, as in
% \author{Author 1 \\ \addr{Address line} \\  ... \\ \addr{Address line}
%         \AND
%         Author 2 \\ \addr{Address line} \\ ... \\ \addr{Address line} \And
%         Author 3 \\ \addr{Address line} \\ ... \\ \addr{Address line}}

% The \author macro works with any number of authors. There are two commands
% used to separate the names and addresses of multiple authors: \And and \AND.
%
% Using \And between authors leaves it to \LaTeX{} to determine where to break
% the lines. Using \AND forces a linebreak at that point. So, if \LaTeX{}
% puts 3 of 4 authors names on the first line, and the last on the second
% line, try using \AND instead of \And before the third author name.

\newcommand{\fix}{\marginpar{FIX}}
\newcommand{\new}{\marginpar{NEW}}

%\iclrfinalcopy % Uncomment for camera-ready version, but NOT for submission.
\begin{document}

\input{appendix_body.tex}

\input{training_examples.tex}

\end{document}
